# Supplementary material for: First principles investigation of exchange interactions in quasi-one-dimensional antiferromagnet CaV2O4
Source: arXiv:1410.7136 source file (2014-10-27)
Supplement: Supplementary file 1 [file SM.pdf]

# Supplementary material to: First principles investigation of exchange interactions in quasi-one-dimensional antiferromagnet $CaV_2O_4$.

Z.V. Pchelkina[1,2,*] and I. V. Solovyev[2,3,†]

[1]*Institute of Metal Physics, S.Kovalevskoy St. 18, 620990 Ekaterinburg, Russia*

[2]*Ural Federal University, Mira St. 19, 620002 Ekaterinburg, Russia*

[3]*Computational Materials Science Unit,*
*National Institute for Materials Science,*
*1-1 Namiki, Tsukuba, Ibaraki 305-0044, Japan*

PACS numbers: 71.20.-b, 71.70.Gm, 75.30.Et

# I. CRYSTAL STRUCTURE DETAILS

TABLE I: Atomic positions for $CaV_2O_4$ in the monoclinic $P2_1/n11$ space group taken from Ref.[1] and transformed into conventional setting.

| atom | $x$ | $y$ | $z$ |
|---|---|---|---|
| V1 | 0.2557 | 0.4324 | 0.6116 |
| V2 | 0.2532 | 0.4198 | 0.1047 |
| O1 | 0.250 | 0.2093 | 0.1642 |
| O2 | 0.254 | 0.1197 | 0.4757 |
| O3 | 0.252 | 0.5206 | 0.7813 |
| O4 | 0.243 | 0.4183 | 0.4275 |
| Ca | 0.25 | 0.7557 | 0.6548 |

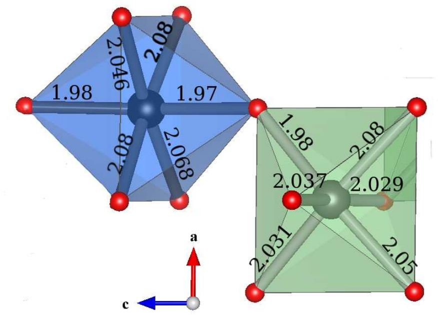


FIG. 1: (Color online). Interatomic V-O distances (Å) for oxygen octahedra around V1 (blue) and V2 (green) atoms in monoclinic structure of $CaV_2O_4$.

# II. HOPPING INTEGRALS AND EXCHANGE INTERACTIONS

TABLE II: Interatomic V-V distances (Å) for $CaV_2O_4$ in the low temperature monoclinic ($P2_1/n11$) and high temperature orthorhombic ($Pnam$) phases.

| bond | notation | Monoclinic ($P2_1/n11$) | Orthorhombic ($Pnam$) |
|---|---|---|---|
| V1-V1 | $d_1^-$ | 3.079 | 3.095 |
| V1-V1 | $d_1^+$ | 3.077 | 3.095 |
| V2-V2 | $d_2^+$ | 3.064 | 3.054 |
| V2-V2 | $d_2^-$ | 3.075 | 3.054 |
| V1-V1 | $d_1^l$ | 2.998 | 3.006 |
| V2-V2 | $d_2^l$ | 2.998 | 3.006 |

TABLE III: Matrices of transfer integrals $t_{i,j}^{m,m'}$ (second column) and exchange interactions between nearest neighbor V ions. Numbers $i$ and $j$ denote the vanadium sites V1 or V2, $m$ runs over the crystal field orbitals $\phi_i^1$, $\phi_i^2$ and $\phi_i^3$. $J_{i,j}^{m,m'}$(SE) (third column) – matrices of exchange interactions obtained within superexchange theory. The sum of all elements of such a matrix is $J$(SE) (fourth column). $J$ (fifth column) are the exchange integrals derived within Hartree-Fock calculation for AFM3 magnetic state. The minus sign corresponds to the AFM interaction. All values are in meV.

| | Hopping matrix $t_{i,j}^{m,m'}$ | $J_{i,j}^{m,m'}$(SE) matrix | $J$(SE) | $J$ |
|---|---|---|---|---|
| $J_1^l$ | $\begin{pmatrix} -265 & 3 & 41 \\ -92 & 63 & 0 \\ 55 & 20 & 71 \end{pmatrix}$ | $\begin{pmatrix} -17.39 & -0.00 & 0.25 \\ -2.09 & -0.97 & 0.00 \\ 0.44 & 0.06 & 0.00 \end{pmatrix}$ | -19.7 | -19.9 |
| $J_2^l$ | $\begin{pmatrix} -233 & 50 & -42 \\ -49 & 66 & 112 \\ 60 & 41 & 67 \end{pmatrix}$ | $\begin{pmatrix} -13.25 & -0.60 & 0.26 \\ -0.59 & -1.05 & 1.85 \\ 0.52 & 0.24 & 0.00 \end{pmatrix}$ | -12.62 | -13.9 |
| $J_1^+$ | $\begin{pmatrix} 43 & -15 & 86 \\ -15 & -111 & -12 \\ 86 & -12 & 16 \end{pmatrix}$ | $\begin{pmatrix} -0.46 & -0.05 & 1.08 \\ -0.05 & -3.05 & 0.02 \\ 1.08 & 0.02 & 0.00 \end{pmatrix}$ | -1.40 | -1.3 |

TABLE IV: Continuation of Tab. III.

| | Hopping matrix $t_{i,j}^{m,m'}$ | $J_{i,j}^{m,m'}$(SE) matrix | $J$(SE) | $J$ |
|---|---|---|---|---|
| $J_1^-$ | $\begin{pmatrix} 2 & 80 & 50 \\ 80 & -32 & 65 \\ 50 & 65 & -14 \end{pmatrix}$ | $\begin{pmatrix} -0.00 & -1.56 & 0.37 \\ -1.56 & 0.25 & 0.62 \\ 0.37 & 0.02 & 0.00 \end{pmatrix}$ | -1.40 | -0.4 |
| $J_2^+$ | $\begin{pmatrix} 78 & 15 & 67 \\ 15 & -82 & 27 \\ 67 & 27 & 50 \end{pmatrix}$ | $\begin{pmatrix} -1.46 & -0.06 & 0.66 \\ -0.06 & -1.62 & 0.11 \\ 0.66 & 0.11 & 0.00 \end{pmatrix}$ | -1.66 | -1.6 |
| $J_2^-$ | $\begin{pmatrix} 69 & 81 & 11 \\ 81 & 56 & 25 \\ 11 & 25 & -53 \end{pmatrix}$ | $\begin{pmatrix} -1.14 & -1.58 & 0.02 \\ -1.58 & 0.75 & 0.09 \\ 0.02 & 0.09 & 0.00 \end{pmatrix}$ | -4.85 | -1.6 |
| $J_c^+$ | $\begin{pmatrix} -4 & -2 & 34 \\ -73 & 5 & 32 \\ -68 & -35 & 194 \end{pmatrix}$ | $\begin{pmatrix} -0.00 & -0.00 & 0.17 \\ -1.32 & -0.01 & 0.15 \\ 0.68 & 0.18 & 0.00 \end{pmatrix}$ | -0.16 | 1.1 |
| $J_c^-$ | $\begin{pmatrix} -19 & 28 & 6 \\ 42 & 54 & -18 \\ -91 & 172 & -14 \end{pmatrix}$ | $\begin{pmatrix} -0.10 & -0.19 & 0.00 \\ -0.43 & -0.71 & 0.05 \\ 1.22 & 4.36 & 0.00 \end{pmatrix}$ | 4.22 | 2.9 |
| $J_b^+$ | $\begin{pmatrix} -11 & 64 & -15 \\ 4 & 77 & 35 \\ 71 & -93 & -16 \end{pmatrix}$ | $\begin{pmatrix} -0.03 & -1.02 & 0.03 \\ -0.00 & -1.47 & 0.18 \\ 0.74 & 1.27 & 0.00 \end{pmatrix}$ | 0.31 | -1.3 |
| $J_b^-$ | $\begin{pmatrix} -10 & 2 & 71 \\ 10 & -22 & -84 \\ 67 & 8 & -57 \end{pmatrix}$ | $\begin{pmatrix} -0.02 & -0.00 & 0.74 \\ -0.02 & -0.12 & 1.03 \\ 0.66 & 0.01 & 0.00 \end{pmatrix}$ | 2.27 | 1.5 |

TABLE V: Main parameters of interatomic magnetic interactions for monoclinic $CaV_2O_4$, calculated in FM and three AFM configurations (see figure 5 of the main text for definition of the different AFM configurations). The total energies performed relative to the energy of AFM3 magnetic state and are normalized to one formula unit. All values are in meV.

| | FM (meV) | AFM1 | AFM2 | AFM3 |
|---|---|---|---|---|
| $J_1^l$ | -22.9 | -20.0 | -20.5 | -19.9 |
| $J_2^l$ | -10.1 | -13.6 | -13.7 | -13.9 |
| $J_1^+$ | -1.6 | -1.4 | -1.7 | -1.3 |
| $J_1^-$ | -0.9 | -0.5 | -0.8 | -0.4 |
| $J_2^+$ | -1.1 | -1.6 | -1.6 | -1.6 |
| $J_2^-$ | 1.2 | -1.4 | -0.8 | -1.6 |
| $J_c^+$ | 2.7 | 1.3 | 1.3 | 1.1 |
| $J_c^-$ | 3.4 | 3.0 | 2.8 | 2.9 |
| $J_b^+$ | -1.2 | -1.5 | -1.2 | -1.3 |
| $J_b^-$ | 1.1 | 1.5 | 1.4 | 1.5 |
| $E_{tot}$ | 73.8 | 1.4 | 6.3 | 0 |

TABLE VI: Parameters of interatomic magnetic interactions (meV) obtained from inelastic neutron scattering (INS) in Ref.[1] (second column), estimated from the fit of the Heisenberg model to the magnetic susceptibility data (SC) in Ref.[2,3] in assumption of two equivalent zigzag chains (third and fourth column) and calculated in present work for AFM3 state (fifth column). The two sets of exchange interactions in fourth column correspond to the two solutions found in Ref.[3]. The minus sign corresponds to the AFM interaction.

| | $J$(INS)[a] | $J$(SC)[b] | $J$(SC)[c] | Present work, AFM3 |
|---|---|---|---|---|
| $J_1^l$ | -30 | 0 | -0.75 /-18.6 | -19.9 |
| $J_2^l$ | -30 | 0 | -0.75 /-18.6 | -13.9 |
| $J_1^+$ | -11 | -19.82 | -19.85/-3.02 | -1.3 |
| $J_1^-$ | -7.9 | -19.82 | -19.85/-3.02 | -0.4 |
| $J_2^+$ | 7.8 | -19.82 | -19.85/-3.02 | -1.6 |
| $J_2^-$ | 5.7 | -19.82 | -19.85/-3.02 | -1.6 |
| $J_c^+$ | -2 | $J_\perp \geqslant 0.9$ | | 1.1 |
| $J_c^-$ | -2 | | | 2.9 |
| $J_b^+$ | -1.5 | | | -1.3 |
| $J_b^-$ | -1.5 | | | 1.5 |

[a]Data from Ref.[1].
[b]Data from Ref.[2].
[c]Data from Ref.[3].


* Electronic address: pzv@ifmlrs.uran.ru

† Electronic address: SOLOVYEV.Igor@nims.go.jp



1 Pieper O *Ph.D. thesis* Der Technischen Universität Berlin (2010)

2 Niazi A *et al.* 2009 *Phys. Rev. B* **79** 104432

3 Pieper O *et al.* 2009 *Phys. Rev. B* **79** 180409
